# Supplementary material for: Constructing a Good Behavior Basis for Transfer using Generalized Policy Updates
Source: arXiv:2112.15025 source file (2022-03-14)

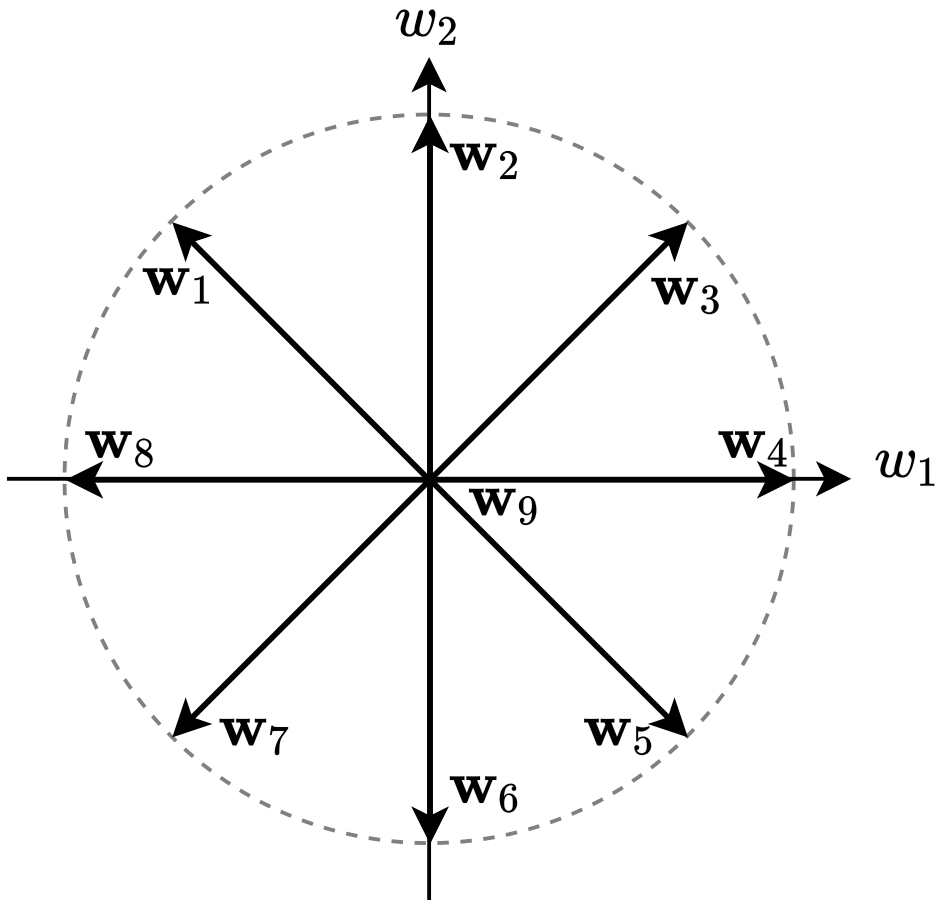

Supplement: Supplementary file 1 [file 2Dplane_supp.pdf]
